# Supplementary material for: Nesterov's method with decreasing learning rate leads to accelerated stochastic gradient descent
Source: arXiv:1908.07861 source file (2020-09-01)
Supplement: Supplementary file 1 [file N2N_appendix_GD.tex]

%appendix application GD

\section{Gradient descent}
\label{appendix: GD}

\subsection{Proof of Proposition \ref{lem: condition GD lyapunov function}}

\begin{itemize}
\item In the convex case, we first start to look for \eqref{Liap_Cond}:
\begin{align*}
\partial_t E^c(t,z) &-  \nabla E^c(t,z)\nabla f(z) \\
&  =  f(z) -f^* - \langle t\nabla f(z) + z-x^* , \nabla f(z) \rangle \\
& = f(z) -f^* - \langle z-x^* , \nabla f(z) \rangle - t|\nabla f(z)  |^2\\
&\leq - t|\nabla f(z)  |^2, 
\end{align*}
by convexity, which gives $r_{E^c} =0$ and $a_{E^c}=t$. Now, by $1$-convexity of the quadratic term and $L$-smoothness of $f$,
\begin{align*}
E^c(t_{k+1}, z_{k+1}) &- E^c(t_k,z_k) \\
& \leq   t_{k+1}(f(z_{k}) - f^* +\langle \nabla f(z_k), z_{k+1} -z_k \rangle 
+\frac{L}{2}|z_{k+1} -z_k|^2 ) -t_k (f(z_{k}) -f^*)\\
& + \frac{1}{2}|z_{k+1} - x^* |^2 - \frac{1}{2}|z_k - x^* |^2\\
& \leq  \langle t_k\nabla f(z_k) + z_k-x^* , z_{k+1} -z_k \rangle + \frac{Lt_{k+1} +1}{2}|z_{k+1} -z_k|^2 
\\& +(t_{k+1}-t_k) (f(z_{k}) -f^*) +(t_{k+1}-t_k)\langle \nabla f(z_k) , z_{k+1}-z_k \rangle \\
& \leq (t_{k+1}-t_k) \partial_t E^c(t_k,z_k) + \langle \nabla E^c(t_k,z_k)  , z_{k+1} -z_k \rangle + \frac{Lt_{k+1} +1}{2}|z_{k+1} -z_k|^2, 
\end{align*}
since, by \eqref{eq: GD},
\[
(t_{k+1}-t_k)\langle \nabla f(z_k) , z_{k+1}-z_k \rangle  \leq 0.
\]
Then $L_{E^c}= Lt_{k+1} +1$.

\item In the strongly convex case, 

\begin{align*}
\partial_t E^{sc}(z) -  \nabla E^{sc}(z)\nabla f(z)  
 &= -\langle \nabla f(z) + \mu(z-x^*) , \nabla f(z) \rangle \\
& = -\mu \langle z-x^* , \nabla f(z) \rangle - |\nabla f(z) |^2\\
&\leq  - \mu \left(f(z) - f^* - \frac{\mu}{2}|z-x^*|^2\right)- |\nabla f(z) |^2,
\end{align*}
by strong convexity and then $r_{E^{sc}} =\mu$ and $a_{E^{sc}}=1$. Concerning \eqref{ass: lyap discrete abstract}, since $E^{sc}$ is time independent, \eqref{ass: lyap discrete abstract} is equivalent to $L$-smoothness condition which gives $L_{E^{sc}}= L+\mu$.
\end{itemize}
