# Supplementary material for: Nesterov's method with decreasing learning rate leads to accelerated stochastic gradient descent
Source: arXiv:1908.07861 source file (2020-09-01)
Supplement: Supplementary file 2 [file N2N_appendix_SGD_str_convex.tex]

% Other method using a different I

If $f$ is $\mu$-strongly convex, assume $e$ satisfies
\begin{eqnarray}
\label{ass: integrability e SGD}
\int_0^{+\infty} e^{\mu s} |e(s)| \, ds < +\infty.
\end{eqnarray}
This condition on the error function is classical \blue{Citations?? Robbins?} %\cite{Robbins}. 
The case $e=0$ is satisfied trivially and corresponds to the gradient descent ODE. \\
Define the augmented Lyapunov function $\tilde{E}^{sc} \, : \, [0,+\infty )  \times {\R}^d \rightarrow [0,+\infty )$ by
$$ \tilde{E}^{sc}(t,x) = E^{sc}(x) + I^{sc}(t),$$
where,
$$ I^{sc}(t) = e^{-\mu t} \int_0^t e^{\mu s} \langle x(s) - x^*, e(s) \rangle \, ds.$$
Then the following result holds.
\begin{proposition}
\label{prop: rate SGD strongly convex}
Let $x$ be a solution of \eqref{eq: SGD convex} with initial data $x_0$ and suppose that $e$ satisfies \eqref{ass: integrability e SGD}. Then,
$$ \frac{d }{dt}\tilde{E}^{sc}(t,x(t)) \leq -\mu \tilde{E}^{sc}(t,x(t)).$$
In addition, $\sup_{t\geq 0} |x(t) - x^*| < +\infty$ and 
$$ \frac{1}{2}|x-x^*|^2 \leq e^{-\mu t} \left( \frac{1}{2}|x_0 -x^*|^2 + I_\infty\right),$$
where,
$$I_\infty:=\sup_{s \geq 0} |x(s) -x^*|\int_0^{+\infty} e^{\mu s} |e(s) | \,ds<+\infty .$$

\end{proposition}

\begin{proof}
For all $t>0$, 
\begin{eqnarray*}
 \frac{d }{dt}\tilde{E}^{sc}(t,x(t)) & =  &- \langle x - x^*, \nabla f(x) \rangle -   \langle x - x^*, e \rangle - \mu I(t) +\langle x - x^*, e \rangle\\
 &\leq & - \frac{\mu}{2}|x -x^*|^2 - \mu I^{sc}(t) = -\mu \tilde{E}^{sc}(t,x).
\end{eqnarray*}
Therefore $\tilde{E}^{sc}(t,x(t))$ is decreasing and then for all $t>0$,
$$ \frac{1}{2}|x(t) - x^* | ^2 \leq \frac{1}{2} |x_0 -x^*| + \int_0^t |x(s)-x^*| e^{\mu s} |e(s)| \,ds.$$
By Gronwall Lemma and \eqref{ass: integrability e SGD}, we deduce that $\sup_{t\geq 0} |x - x^*| < +\infty$ and the proof is concluded.
\end{proof}

Define the discrete time augmented Lyapunov function $\tilde{E}^{sc}_k$, for $k \geq 1$, by 
$$ \tilde{E}^{sc}_k = E^{sc}(x_k) + I^{sc}_k,$$
where $x_k$ is generated by the forward Euler discretization of \eqref{eq: SGD convex}, \eqref{eq: dicrete SGD convex}, and 
$$ I^{sc}_k= (1 - h\mu)^k h\sum_{i=0}^k (1 - h\mu)^{-i} \langle x_i -x^*, e_{i-1} \rangle,$$
with the notation $e_{-1}=0$.\\
Assume $e_k$ satisfies 
\begin{equation}
\label{ass: e_k SDE str convex}
\sum_{k=0}^{+\infty} (1-h\mu)^{-k}|e_k| < +\infty.
\end{equation}

%\blue{
\begin{remark}
Condition \eqref{ass: e_k SDE str convex} is the discretization of the continuous condition \eqref{ass: integrability e SGD}.
\end{remark}
%}

\begin{proposition}
Assume that $h \leq \frac{1}{L}$ and $e_k$ satisfies \eqref{ass: e_k SDE str convex}. Then,
$$ \tilde{E}^{sc}_{k+1} \leq (1- h\mu) \tilde{E}^{sc}_k.$$
In addition, $\sup_{i\geq 1} |x_i -x^*| < +\infty$ and we deduce,
$$ \frac{1}{2}|x_k - x^*|^2 \leq (1 -h\mu)^k \left( \frac{1}{2}|x_0 -x^*|^2 + I_\infty\right),$$
where,
$$ I_\infty := h\sup_{i\geq 1} |x_i -x^*| \sum_{i=0}^{+\infty} (1 - h\mu)^{-i-1} |e_{i} | <+\infty.$$

\end{proposition}

\begin{proof}
First, as usual, we have
\begin{eqnarray*}
\frac{1}{2}|x_{k+1} - x^*|^2 -\frac{1}{2}|x_{k} - x^*|^2 & =&  -h\langle \nabla f(x_k) ,x_k -x^* \rangle - h \langle e_k ,x_k -x^* \rangle + \frac{h^2}{2} |\nabla f(x_k) +e_k|^2\\
&\leq & -\frac{h\mu }{2} |x_k -x^* |^2 +h(f^* -f(x_k))+ \frac{h^2}{2} |\nabla f(x_k) +e_k|^2\\
&\leq & -\frac{h\mu }{2} |x_k -x^* |^2 -\frac{h}{2L}|\nabla f(x_k) |^2 + \frac{h^2}{2} |\nabla f(x_k) +e_k|^2.
\end{eqnarray*}
In addition,
\begin{eqnarray*}
I^{sc}_{k+1} - I^{sc}_k &=& h(1-h\mu )^k \left( (1- h\mu)\sum_{i=0}^{k+1} (1-h\mu)^{-i}\langle x_i -x^*, e_{i-1} \rangle - \sum_{i=0}^{k} (1-h\mu)^{-i}\langle x_i -x^*, e_{i-1}\rangle \right)\\
& = & -h \mu I_k^{sc} + h \langle x_{k+1} -x^*, e_k \rangle.
\end{eqnarray*}
Combining these two inequalities,
\begin{eqnarray*}
\tilde{E}^{sc}_{k+1} -\tilde{E}^{sc}_k &\leq & -h \mu \tilde{E}^{sc}_k +h \langle x_{k+1} -x_k, e_k \rangle  -\frac{h}{2L}|\nabla f(x_k) |^2 + \frac{h^2}{2} |\nabla f(x_k) +e_k|^2\\
& \leq & -h \mu \tilde{E}^{sc}_k + \frac{h}{2}\left(h -\frac{1}{L} \right) |\nabla f(x_k) |^2 -\frac{h^2}{2}|e_k|^2\\
& \leq &  -h \mu \tilde{E}^{sc}_k,
\end{eqnarray*}
when $h \leq \frac{1}{L}$.\\

In order to conclude, we also need to establish that $\tilde{E}^{sc}_k$ is bounded below.  That follows from discrete Gronwall's inequality, as was already done in the continuous case in Proposition \ref{prop: rate SGD strongly convex}.
\end{proof}

\end{itemize}
