# Supplementary material for: Nesterov's method with decreasing learning rate leads to accelerated stochastic gradient descent
Source: arXiv:1908.07861 source file (2020-09-01)
Supplement: Supplementary file 4 [file N2N_appendix_acc_convec.tex]

% Appendix acceleration convergence convex

\section{Accelerated rate: convex case}
\label{appendix: acc convex}

\subsection{ODE and derivation of Nesterov's method}
\paragraph{Derivation of \eqref{OurEqnCC}}
Solve for $v$ in the first line of \eqref{NODE}
\[
 v = \frac{t}{2} (\dot{x} +\frac{1}{\sqrt{L}}\nabla f(x)) + x
 \]
differentiate to obtain
\[ \dot{v}=\frac{1}{2} (\dot{x} +\frac{1}{\sqrt{L}}\nabla f(x)) +\frac{t}{2} (\ddot{x} +\frac{1}{\sqrt{L}} D^2 f(x) \cdot \dot{x} ) + \dot{x}.
\]
Insert into the second line of \eqref{NODE}
\[
\frac{1}{2} (\dot{x} +\frac{1}{\sqrt{L}}\nabla f(x)) +\frac{t}{2} (\ddot{x} +\frac{1}{\sqrt{L}} D^2 f(x) \cdot \dot{x} ) + \dot{x} 
=  -\frac{t}{2} \nabla f(x).
\]
Simplify to obtain \eqref{OurEqnCC}.

\paragraph{Proof of Proposition \ref{prop: discret Nest convex}}
The system \eqref{FEg} with  a constant time step $h_k=\frac{1}{\sqrt{L}}$ gives $t_k = h(k+2)=\frac{k+2}{\sqrt{L}}$  and
\begin{equation*}	
\begin{cases}
x_{k+1} - x_k &= \frac{2}{k+2}(v_k -x_k) -\frac{1}{L}\nabla f(y_k)\\
v_{k+1} - v_k &= -\frac{k+2}{2L}\nabla f(y_k) 
\end{cases}
\end{equation*}
Using \eqref{FEg} gives
\[
x_{k+1} = y_k -\frac{1}{L}\nabla f(y_k)
\]
the first equation in \eqref{sys: Nesterov convex}.  For the second equation in the system above, eliminate the gradient term using the first equation to obtain
\[
v_{k+1} = \frac{k+2}2(x_{k+1}-x_k) + x_k
\]
Using the definition of $y_k$ in \eqref{FEg}, applied at $k+1$, and solve for the variable $v_{k+1}$ to give 
\[
v_{k+1} = \frac {k+3}2 y_{k+1} - \frac {k+1} 2 x_{k+1}.
\]
Combine the last to equations to obtain the second equation in~\eqref{sys: Nesterov convex}.

\subsection{Lyapunov analysis for \eqref{NODE}}
\label{appendix: acc convex lyap analysis continusous unperturbed}

\begin{proposition}\label{Thm:ConvexLiapNoAcc}
Suppose $f$ is convex and $L$-smooth. 
Let $x,v$ be solutions of \eqref{NODE} and let $E^{ac,c}$ be given by \eqref{LiapCTS}.
Then $E^{ac,c}$ is a  continuous Lyapunov function  with $r_{E^{ac,c}} =0$ and $a_{E^{ac,c}} = \frac{ t^2}{\sqrt{L}} $ (with gap $t^2|\nabla f(x)|^2$) i.e.
\[
 \frac{d }{dt}E^{ac,c}(t,x(t),v(t);0) \leq -\frac{ t^2}{\sqrt{L}}  |\nabla f(x) |^2 .
 \]
%and $E_k^{ac,c}$ is a discrete Lyapunov function, with $L_{E^{ac,c}}=t_k^2$, for the sequence generated by \eqref{FEg}, for all $k\geq 0$, 
%\[
%E_{k+1}^{ac,c} \leq E_k^{ac,c} -h^2(f(x_k) - f^*) + \left( h - \frac{1}{\sqrt{L}} \right) t_k^2h |\nabla f(y_k) |^2,
%\] 
%for $h \leq \frac{1}{ \sqrt{L}}$.
\end{proposition}

%\blue{TODO merge this one to previous one } 

%Can say : we show we get Nesterov, so part of the proof is done. 
%The main step is the discretization.  Also include the proof in continous time.
 
% Since   \eqref{FEg} is equivalent to Nesterov's method, the rate is known. The proof of the rate using a Lyapunov function can be found in \cite{beck2009fast}. A proof which shows that we can use the constant time step can be found in~ \cite{beck2017first}. 
%Notice that the discrete Lyapunov function 
% \eqref{Ek_defn} was used in \cite{su2014differential,attouch2016fast} to prove a rate.  

%\begin{remark}
%	Note, compared to Su-Boyd-Cand\'es' ODE \eqref{ODE_Su}, there is a gap in the dissipation of the Lyapunov function $E^{ac,c}$, which will not be there if the extra term, $-\frac{1}{\sqrt{L}}\nabla f(x)$, was missing.  In particular, if $\tilde z$ solution of \eqref{ODE_Su}, and $z$ solution of \eqref{NODE}, then we can prove  faster convergence due to the gap. Indeed, this gap permits to improve the asymptotic rate of the descent of the gradient, see Corollary \ref{cor: decrease gradient}.    
%\end{remark} 
 
\begin{corollary}
\label{prop: rate convex continuous }
Let $f$ be a convex and $L$-smooth function. 
Let $(x(t),v(t))$ be a solution to \eqref{NODE}, then for all $t>0$,
\[
f(x(t)) - f^* \leq \frac{2}{ t^2} |v_0 -x^* |^2.
\]
%Furthermore, let $x_k,v_k$ be given by \eqref{FEg}. Then for all $k\geq 0$ and $h =\frac{1}{ \sqrt{L}}$,
%\[
%f(x_k) - f^* \leq \frac{ 1 }{(k+1)^2}\left( f(x_0) - f^* + 2L |v_0-x^*|^2\right).
%\]
\end{corollary}

 %The proof of the continuous time part is short, and so we include it here. 
\begin{proof}[Proof of Proposition~\ref{Thm:ConvexLiapNoAcc}]
First, by definition of $E^{ac,c}$, we have
\begin{align*}
\frac{d }{dt}E^{ac,c}(t,x(t),v(t))  
&\leq    2t(f(x) - f^*) + t^2 \langle \nabla f(x) , \dot{x} \rangle + 4\langle v - x^* , \dot{v} \rangle \\
&\leq  2t( f(x) - f^*)  +2 t  \langle \nabla f(x) , v - x \rangle - \frac{ t^2}{\sqrt{L}}|\nabla f(x) |^2  -2t  \langle v - x^*, \nabla f(x) \rangle\\
& \leq  2t ( f(x) - f^* - \langle x - x^* , \nabla f(x) \rangle )  - \frac{ t^2}{\sqrt{L}} |\nabla f(x) |^2. 
\end{align*}
The proof is concluded by convexity, 
\[ f(x) - f^* - \langle x - x^* , \nabla f(x) \rangle \leq 0. \qedhere
\]

\end{proof}

\subsection{Classical inequality in the perturbed case}
\label{appendix:inequality dissipation perturbed convex acc}
Before proving Proposition \ref{prop: different gaps convex acc perturbed}, using the convexity and the $L$-smoothness of $f$, we prove a gneralization of the classical inequality obtained in \cite{attouch2016fast} or \cite{su2014differential} in the case $e_k=0$:
\begin{align}
\label{eq:dissipation E acc convex pert}
t_k^2(f(x_{k+1} - f^*) &- t_{k-1}^2(f(x_{k} - f^*) \nonumber\\
&\leq -h^2 (f(x_k) -f^*) + 2ht_k\langle \nabla f(y_k),v_k -x^*  \rangle  -\left(\frac{1}{\sqrt{L}} -\frac{h}{2}\right)h t_k^2|\nabla f(y_k) |^2 \nonumber\\
 &-\frac{ht_k^2}{\sqrt{L}}\langle \nabla f(y_k), e_k \rangle +h^2 t_k^2\left\langle \nabla f(y_k) +\frac{e_k}{2},e_k \right\rangle.
\end{align}

The proof is a perturbed version of the one in \cite{beck2009fast,su2014differential,attouch2016fast}. First we prove the following inequality:
\begin{lemma}
Assume $f$ is a convex, $L$-sùoothness function. For all $x,y,z$, $f$ satisfies
\begin{equation}
\label{eq: ineq 3 points}
f(z) \leq f(x) +\langle \nabla f(y), z-x \rangle +\frac{L}{2}|z-y|^2.
\end{equation}
\end{lemma}

\begin{proof}
By $L$-smoothness, 
\[
f(z) - f(x) \leq f(y) - f(x)  + \langle \nabla f(y) , z-y \rangle +\frac{ L}{2}|z-y|^2.
\]
and since $f$ is convex, 
\[
f(y) - f(x) \leq \langle \nabla f(y) , y -x \rangle.
\]
We conclude the proof combining these two inequalities.
\end{proof}

Now apply inequality \eqref{eq: ineq 3 points} at $(x,y,z)=(x_k,y_k, x_{k+1})$:  
\begin{align*}
f(x_{k+1})  
& \leq  f(x_k) +\langle \nabla f(y_k), x_{k+1}-x_k \rangle +\frac{L}{2}|x_{k+1}-y_k|^2\\
& \leq  f(x_k) +\frac{2h}{t_k}\langle \nabla f(y_k), v_k -x_k \rangle -\frac{h}{\sqrt{L}}|\nabla f(y_k) |^2  -\frac{h}{\sqrt{L}}\langle \nabla f(y_k), e_k \rangle + \frac{h^2}{2}|\nabla f(y_k) +e_k|^2,
\end{align*}
and then
\begin{multline}
\label{eq: inq 1}
f(x_{k+1}) \leq  f(x_k) +\frac{2h}{t_k}\langle \nabla f(y_k), v_k -x_k \rangle -\left(\frac{1}{\sqrt{L}} -\frac{h}{2}\right)h |\nabla f(y_k) |^2\\
-\frac{h}{\sqrt{L}}\langle \nabla f(y_k), e_k \rangle + h^2\left\langle \nabla f(y_k) +\frac{e_k}{2},e_k \right\rangle.
\end{multline}

If we apply \eqref{eq: ineq 3 points} also at $(x,y,z)=(x^*,y_k, x_{k+1})$ we obtain
\begin{align*}
f(x_{k+1})  &\leq  f^* +\langle \nabla f(y_k), x_{k+1}-x^* \rangle +\frac{L}{2}|x_{k+1}-y_k|^2\\
& \leq  f^* +\langle \nabla f(y_k), y_k -x^* \rangle -\frac{h}{\sqrt{L}}|\nabla f(y_k) |^2  -\frac{h}{\sqrt{L}}\langle \nabla f(y_k), e_k \rangle + \frac{h^2}{2}|\nabla f(y_k) +e_k|^2
\end{align*}
then,
\begin{multline}
\label{eq: inq 2}
f(x_{k+1})  \leq  f^* +\langle \nabla f(y_k), y_k -x^* \rangle -\left(\frac{1}{\sqrt{L}} 
-\frac{h}{2}\right)h |\nabla f(y_k) |^2\\
-\frac{h}{\sqrt{L}}\langle \nabla f(y_k), e_k \rangle +h^2 \left\langle \nabla f(y_k) +\frac{e_k}{2},e_k \right\rangle.
\end{multline}

Summing $\left( 1 - \frac{2h}{t_k}\right)$\eqref{eq: inq 1} and $\frac{2h}{t_k}$\eqref{eq: inq 2}, we have
\begin{align*}
f(x_{k+1}) -f^* & \leq   \left( 1- \frac{2h}{t_k} \right)(f(x_k) -f^*)  + \frac{2h}{t_k}\langle \nabla f(y_k),v_k -x^*  \rangle \\
& -\left(\frac{1}{\sqrt{L}} -\frac{h}{2}\right)h |\nabla f(y_k) |^2    -\frac{h}{\sqrt{L}}\langle \nabla f(y_k), e_k \rangle  +h^2 \left\langle \nabla f(y_k) +\frac{e_k}{2},e_k \right\rangle.
\end{align*} 
Then,
\begin{align*}
t_k^2(f(x_{k+1}) -f^*) &\leq  \left( t_k- 2h \right)t_k(f(x_k) -f^*) + 2ht_k\langle \nabla f(y_k),v_k -x^*  \rangle  \\
&-\left(\frac{1}{\sqrt{L}} -\frac{h}{2}\right)h t_k^2|\nabla f(y_k) |^2   -\frac{ht_k^2}{\sqrt{L}}\langle \nabla f(y_k), e_k \rangle \\
&+h^2 t_k^2\left\langle \nabla f(y_k) +\frac{e_k}{2},e_k \right\rangle\\
&\leq  \left( t_{k-1}^2- h^2 \right)(f(x_k) -f^*) + 2ht_k\langle \nabla f(y_k),v_k -x^*  \rangle \\
& -\left(\frac{1}{\sqrt{L}} -\frac{h}{2}\right)h t_k^2|\nabla f(y_k) |^2   -\frac{ht_k^2}{\sqrt{L}}\langle \nabla f(y_k), e_k \rangle \\
&+h^2 t_k^2\left\langle \nabla f(y_k) +\frac{e_k}{2},e_k \right\rangle,
\end{align*}
which concludes the proof.

\subsection{Proof of Proposition \ref{prop: different gaps convex acc perturbed}}

By definition of $v_{k+1}$, we have
\begin{align*}
2|v_{k+1} -x^* |^2 &-  2|v_{k} -x^* |^2 \\
&=  -2ht_k \langle v_k -x^*, \nabla f(y_k) +e_k \rangle + \frac{h^2t_k^2}{2}|\nabla f(y_k) +e_k |^2\\
& =  -2ht_k \langle v_k -x^*, \nabla f(y_k) + \frac{h^2t_k^2}{2}|\nabla f(y_k)|^2 \\
& -2ht_k \langle v_k -x^*, e_k \rangle  + h^2t_k^2\left\langle \nabla f(y_k) +\frac{e_k}{2},e_k \right\rangle. 
\end{align*}
Therefore, combining it with \eqref{eq:dissipation E acc convex pert} from Appendix \ref{appendix:inequality dissipation perturbed convex acc}, we obtain
\begin{align*}
E_{k+1}^{ac,c}  - E_k^{ac,c}   
&\leq  -h^2 (f(x_k) -f^*) -\left(\frac{1}{\sqrt{L}} - h \right)h t_k^2|\nabla f(y_k) |^2 \\
&-2ht_k  \langle v_k -x^* - \frac{t_k}{\sqrt{L}}\nabla f(y_k) , e_k \rangle + 2h^2t_k^2 \left\langle \nabla f(y_k) +\frac{e_k}{2},e_k \right\rangle,
\end{align*}
and \eqref{eq:main inequality E convex acc perturbed} is proved.
