# Supplementary material for: Nesterov's method with decreasing learning rate leads to accelerated stochastic gradient descent
Source: arXiv:1908.07861 source file (2020-09-01)
Supplement: Supplementary file 5 [file N2N_appendix_acc_str_convex.tex]

%N2N_appendix_acc_str_convex

\section{Accelerated rate: strongly convex case}
\label{appendix: acc str convex}

\subsection{ODE and derivation of Nesterov's method}
\label{appendix: derivation second order ODE str convex}

\paragraph{Equivalence between \eqref{NODESC} and \eqref{OurEqnSCC}}
Solve for $v$ in the first line of \eqref{NODESC}
\[
 v = \frac{1}{\sqrt{\mu}} (\dot{x} +\frac{1}{\sqrt{L}}\nabla f(x)) + x
 \]
differentiate to obtain
\[ \dot{v}= \frac{1}{\sqrt{\mu}} (\ddot{x} +\frac{1}{\sqrt{L}}D^2 f(x) \cdot \dot{x}) + \dot{x}.
\]
Insert into the second line of \eqref{NODESC}
\[
\frac{1}{\sqrt{\mu}} (\ddot{x} +\frac{1}{\sqrt{L}}D^2 f(x) \cdot \dot{x}) + \dot{x}
 = -\dot{x} -\left(\frac{1}{\sqrt{L}} +\frac{1}{\sqrt{\mu}}\right) \nabla f(x).
\]
Simplify to obtain \eqref{OurEqnSCC}.

\paragraph{Proof of Proposition \ref{prop: derive Nest str covnex}}
 \eqref{FE-SC} with  $h_k = 1/\sqrt{L}$   becomes
\begin{equation*}
\begin{cases}
x_{k+1} - x_k &= \tfrac{\sqrt{\CCff}}{1 + \sqrt{\CCff}}(v_k -x_k) -\frac{1}{L}\nabla f(y_k)\\
v_{k+1} - v_k &= \tfrac{\sqrt{\CCff}}{1 + \sqrt{\CCff}}(x_k -v_k) -\frac{1}{\sqrt{L\mu}}\nabla f(y_k) 
\end{cases}
\end{equation*}	%\nonumber

Eliminate the variable $v_k$ using the definition of $y_k$ to obtain \eqref{sys: Nesterov str convex}.

\subsection{Lyapunov analysis}
\label{appendix: lyap str convex}
n the next proposition, we show that $E^{ac,c}$ is a rate-generating Lyapunov function, in the sense of Definition \ref{def:reate-gene Lyap abstract}, for system \eqref{NODESC} and its explicit discretization \eqref{FE-SC}. 

\begin{proposition}
\label{thm:lipaunov gap continuous and discrete SC acc}
Suppose $f$ is $\mu$-strongly convex and $L$-smooth. Let $(x,v)$ be a solution of \eqref{NODESC} and $(x_k,v_k)$ be a sequences generated by \eqref{FE-SC}. Let $E^{ac,sc}$ be given by \eqref{eq:Lyapunov function str convex acc}.
Then $E^{ac,sc}$ is a  continuous Lyapunov function  with $r_{E^{ac,sc}} =\sqrt{\mu}$ and $a_{E^{ac,sc}} = \frac{ 1}{\sqrt{L}} $ i.e.
\begin{multline}
\label{eq:lyap gap continuous}
\frac{d }{dt}E^{ac,sc}(x,v) 
\leq - \sqrt{\mu} E^{ac,sc}(x,v) - \frac{1}{\sqrt{L}} |\nabla f(x) |^2 - \frac{\mu \sqrt{\mu}}{2} | v-x |^2.
\end{multline}
\end{proposition}%

Then we retrieve the usual optimal rates in the continuous and discrete cases.
\begin{corollary}
\label{prop: rate str convex continuous acc}
Let $f$ be a $\mu$-strongly convex and $L$-smooth function. 
Let $(x(t),v(t))$ be a solution to \eqref{NODE}, then for all $t>0$,
\[
f(x(t)) - f^* +\frac{\mu}{2} |v(t)-x^*|^2 \leq \exp(-\sqrt{\mu} t)E^{ac,sc}(x_0 , v_0).
\]
\end{corollary}

The proof of Corollary \ref{prop: rate str convex continuous acc} results immedialtly from Proposition \ref{thm:lipaunov gap continuous and discrete SC acc} and then, we focus on the proof of \eqref{eq:lyap gap continuous} in the following.\\

\begin{proof}[Proof of \eqref{eq:lyap gap continuous}]
Using \eqref{NODESC}, we obtain
\begin{align*}
\frac{d }{dt} E^{ac,sc}(x,v) 
& =  \langle \nabla f(x), \dot{x} \rangle +  \sqrt{\mu} \langle v- x^* , \dot{v} \rangle \\ 
&=   \sqrt{\mu} \langle \nabla f(x), v-x \rangle - \frac{1}{\sqrt{L}}|\nabla f(x) |^2 - \mu \sqrt{\mu}\langle v- x^* , v-x \rangle \\
&- \sqrt{\mu} \langle \nabla f(x), v-x^* \rangle = - \sqrt{\mu} \langle \nabla f(x), x-x^* \rangle \\
&- \frac{1}{\sqrt{L}}|\nabla f(x) |^2 - \frac{\mu \sqrt{\mu}}{2} \left[  |v- x^*|^2  + |v-x|^2 - |x-x^*|^2 \right].
\end{align*}
By strong convexity, we have
\begin{align*}
\frac{d }{dt}E^{ac,sc}(x,v) 
& \leq  -\sqrt{\mu} \left( f(x) - f^* +\frac{\mu}{2} |x-x^*|^2 \right) - \frac{1}{\sqrt{L}}|\nabla f(x) |^2\\ 
& - \frac{\mu \sqrt{\mu}}{2} \left[  |v- x^*|^2  + |v-x|^2 - |x-x^*|^2 \right]\\
&\leq  -\sqrt{\mu} E^{ac,sc}(x,v) - \frac{1}{\sqrt{L}}|\nabla f(x) |^2 - \frac{\mu \sqrt{\mu}}{2} |v-x|^2 .\\
\end{align*}
which establishes \eqref{eq:lyap gap continuous}.
\end{proof}

\subsection{Proof of Proposition \ref{thm:Acc GD SC}}
First, arguing as in Proposition \ref{thm:lipaunov gap continuous and discrete SC acc},
\begin{align*}
f(x_{k+1}) -f(x_k) 
& \leq  \langle \nabla f(y_k) , y_k -x_k \rangle - \frac{\mu}{2}|y_k -x_k|^2 \\
&+ \left( \frac{h^2}{2} - \frac{h}{\sqrt{L}}\right) |\nabla f(y_k)|^2  - \frac{h}{\sqrt{L}} \langle \nabla f(y_k) , e_k \rangle + h^2 \left\langle \nabla f(y_k) +\frac{e_k}{2}, e_k \right\rangle,
\end{align*}
and,
\begin{align*}
\frac{\mu}{2}|v_{k+1} - x^* |^2 - \frac{\mu}{2}|v_{k} - x^* |^2 
& \leq  -h\sqrt{\mu}E^{ac,sc}_k + \left( \sqrt{\mu} + Lh \right)\frac{\sqrt{\mu}}{2}|x_k - y_k|^2 + \frac{h^2}{2}|\nabla f(y_k)|^2\\
&- h\sqrt{\mu} \langle v_k -x^* +x_k -y_k, e_k \rangle + h^2 \left\langle \nabla f(y_k) +\frac{e_k}{2}, e_k \right\rangle.
\end{align*}
Summing these two inequalities, 
\begin{align*}
E_{k+1}^{ac,sc}  - E_k^{ac,sc} 
&\leq  - h\sqrt{\mu} E_k^{ac,sc} +\left( h^2 - \frac{h}{\sqrt{L}} \right) |\nabla f(y_k) |^2 \\
&+ \left( \frac{h\sqrt{\mu}L}{2} - \frac{\sqrt{\mu}}{2h}\right) |x_k -y_k|^2    -h \sqrt{\mu} \langle x_k -y_k + v_k -x^*, e_k \rangle \\
&+\frac{h}{\sqrt{L}}\langle \nabla f(y_k), e_k \rangle + 2h^2 \left\langle \nabla f(y_k) +\frac{e_k}{2}, e_k \right\rangle.
\end{align*}
