# Supplementary material for: Nesterov's method with decreasing learning rate leads to accelerated stochastic gradient descent
Source: arXiv:1908.07861 source file (2020-09-01)
Supplement: Supplementary file 6 [file N2N_appendix_ineq_convex_acc.tex]

\section{Proof of inequality \eqref{eq:dissipation E acc convex pert}}
\label{appendix:inequality dissipation perturbed convex acc}

The proof is a perturbed version of the one in \cite{beck2009fast,su2014differential,attouch2016fast}. First we prove the following inequality:

\begin{lemma}
Assume $f$ is a convex, $L$-sùoothness function. For all $x,y,z$, $f$ satisfies
\begin{equation}
\label{eq: ineq 3 points}
f(z) \leq f(x) +\langle \nabla f(y), z-x \rangle +\frac{L}{2}|z-y|^2.
\end{equation}

\end{lemma}

\begin{proof}
By $L$-smoothness, 
\[
f(z) - f(x) \leq f(y) - f(x)  + \langle \nabla f(y) , z-y \rangle +\frac{ L}{2}|z-y|^2.
\]
and since $f$ is convex, 
\[
f(y) - f(x) \leq \langle \nabla f(y) , y -x \rangle.
\]
We conclude the proof comibning these two inequalities.
\end{proof}

Now apply inequality \eqref{eq: ineq 3 points} at $(x,y,z)=(x_k,y_k, x_{k+1})$:  
\begin{eqnarray*}
f(x_{k+1})  & \leq & f(x_k) +\langle \nabla f(y_k), x_{k+1}-x_k \rangle +\frac{L}{2}|x_{k+1}-y_k|^2\\
& \leq & f(x_k) +\frac{2h}{t_k}\langle \nabla f(y_k), v_k -x_k \rangle -\frac{h}{\sqrt{L}}|\nabla f(y_k) |^2\\
&& -\frac{h}{\sqrt{L}}\langle \nabla f(y_k), e_k \rangle + \frac{h^2}{2}|\nabla f(y_k) +e_k|^2,
\end{eqnarray*}
and then
\begin{equation}
\label{eq: inq 1}
f(x_{k+1})  \leq  f(x_k) +\frac{2h}{t_k}\langle \nabla f(y_k), v_k -x_k \rangle -\left(\frac{1}{\sqrt{L}} -\frac{h}{2}\right)h |\nabla f(y_k) |^2\\
-\frac{h}{\sqrt{L}}\langle \nabla f(y_k), e_k \rangle + h^2\left\langle \nabla f(y_k) +\frac{e_k}{2},e_k \right\rangle.
\end{equation}

If we apply \eqref{eq: ineq 3 points} also at $(x,y,z)=(x^*,y_k, x_{k+1})$ we obtain
\begin{eqnarray*}
f(x_{k+1})  & \leq & f^* +\langle \nabla f(y_k), x_{k+1}-x^* \rangle +\frac{L}{2}|x_{k+1}-y_k|^2\\
& \leq & f^* +\langle \nabla f(y_k), y_k -x^* \rangle -\frac{h}{\sqrt{L}}|\nabla f(y_k) |^2\\
&& -\frac{h}{\sqrt{L}}\langle \nabla f(y_k), e_k \rangle + \frac{h^2}{2}|\nabla f(y_k) +e_k|^2
\end{eqnarray*}

then,
\begin{equation}
\label{eq: inq 2}
f(x_{k+1}) \leq  f^* +\langle \nabla f(y_k), y_k -x^* \rangle -\left(\frac{1}{\sqrt{L}} -\frac{h}{2}\right)h |\nabla f(y_k) |^2
  -\frac{h}{\sqrt{L}}\langle \nabla f(y_k), e_k \rangle +h^2 \left\langle \nabla f(y_k) +\frac{e_k}{2},e_k \right\rangle.
\end{equation}

Summing $\left( 1 - \frac{2h}{t_k}\right)$\eqref{eq: inq 1} and $\frac{2h}{t_k}$\eqref{eq: inq 2}, we have
\begin{eqnarray*}
f(x_{k+1}) -f^* & \leq  & \left( 1- \frac{2h}{t_k} \right)(f(x_k) -f^*)  + \frac{2h}{t_k}\langle \nabla f(y_k),v_k -x^*  \rangle  -\left(\frac{1}{\sqrt{L}} -\frac{h}{2}\right)h |\nabla f(y_k) |^2 \\
& &  -\frac{h}{\sqrt{L}}\langle \nabla f(y_k), e_k \rangle +h^2 \left\langle \nabla f(y_k) +\frac{e_k}{2},e_k \right\rangle.
\end{eqnarray*} 
Then,
\begin{eqnarray*}
t_k^2(f(x_{k+1}) -f^*) &\leq & \left( t_k- 2h \right)t_k(f(x_k) -f^*) + 2ht_k\langle \nabla f(y_k),v_k -x^*  \rangle  -\left(\frac{1}{\sqrt{L}} -\frac{h}{2}\right)h t_k^2|\nabla f(y_k) |^2 \\
& &  -\frac{ht_k^2}{\sqrt{L}}\langle \nabla f(y_k), e_k \rangle +h^2 t_k^2\left\langle \nabla f(y_k) +\frac{e_k}{2},e_k \right\rangle\\
&\leq & \left( t_{k-1}^2- h^2 \right)(f(x_k) -f^*) + 2ht_k\langle \nabla f(y_k),v_k -x^*  \rangle  -\left(\frac{1}{\sqrt{L}} -\frac{h}{2}\right)h t_k^2|\nabla f(y_k) |^2 \\
& &  -\frac{ht_k^2}{\sqrt{L}}\langle \nabla f(y_k), e_k \rangle +h^2 t_k^2\left\langle \nabla f(y_k) +\frac{e_k}{2},e_k \right\rangle,
\end{eqnarray*}
which concludes the proof.
